# Supplementary material for: Harvesting nucleating structures in nanoparticle crystallization: The example of gold, silver and iron
Source: arXiv:2401.03969 source file (2024-07-08)
Supplement: Supplementary file 1 [file NucleationInNano_SI.pdf]

# Supporting Information: Harvesting nucleating structures in nanoparticle crystallization: The example of gold, silver and iron

Arthur France-Lanord,*,† Sarath Menon,‡ and Julien Lam*,¶

†*Sorbonne Université, Institut des Sciences du Calcul et des Données, ISCD, F-75005 Paris, France*

‡*Max-Planck-Institut für Eisenforschung GmbH, D-40237 Düsseldorf, Germany*

¶*Univ. Lille, CNRS, INRA, ENSCL, UMR 8207, UMET, Unité Matériaux et Transformations, F 59000 Lille, France*

§*Centre d'élaboration des Matériaux et d'Etudes Structurales, CNRS (UPR 8011), 29 rue Jeanne Marvig, 31055 Toulouse Cedex 4, France*

E-mail: arthur.france-lanord@cnrs.fr; julien.lam@cnrs.fr

## Contents

**1 Disentangling temperature and droplet size effects** **S-2**

**2 Aimless shooting additional figures** **S-3**

**3 Influence of *ad hoc* parameters** **S-3**

# 1 Disentangling temperature and droplet size effects

In order to disentangle the role of nanoparticle size and of temperature, we performed additional simulations, with the same methodology – combining metadynamics, CPA, aimless shooting and a final round of CPA –, for the $N = 2000$ system, yet at the exact same temperature as used for $N = 500$ in all three materials. If the observed change in critical nucleus size is not due to the reduction of the droplet size but only to the change in temperature, these additional results should match the results obtained for $N = 500$. In Fig. S1, we observe that it is not the case. In particular, for each material, the nucleus size is inferior to what was obtained for $N = 500$. The position of the nucleus as well as its degree of crystallinity also change under these new conditions. Altogether, these results suggest that an additional layer of complexity exists upon changing the temperature at a given size, which should be investigated in future work. Meanwhile, this demonstrates that our results do not not simply correspond to a temperature effect, but also capture the influence of the droplet size.

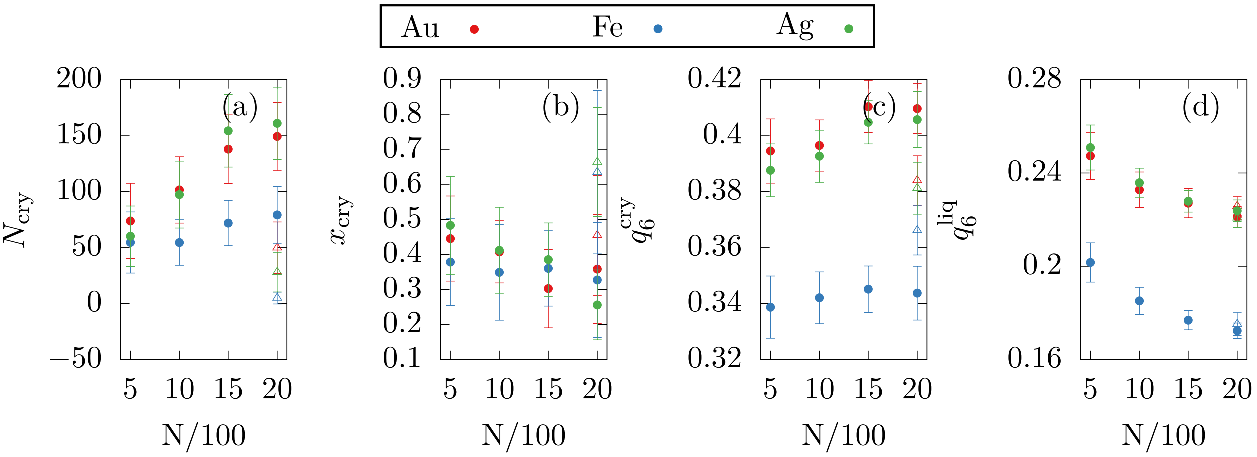


Figure S1: Influence of the droplet size on the structure of the critical structures in terms of the size of the largest crystalline cluster (a), the radial position of the largest crystalline cluster (b), the value of $\overline{q_6}$ averaged over atoms of the largest crystalline cluster (c) and of the remaining atoms (d). In all graphs, filled circles were obtained at a fixed degree of supercooling for each droplet sizes ($T/T_{melt} = 0.85$), and open triangles were obtained at the temperature used for the smallest droplet ($N = 500$).

## 2 Aimless shooting additional figures

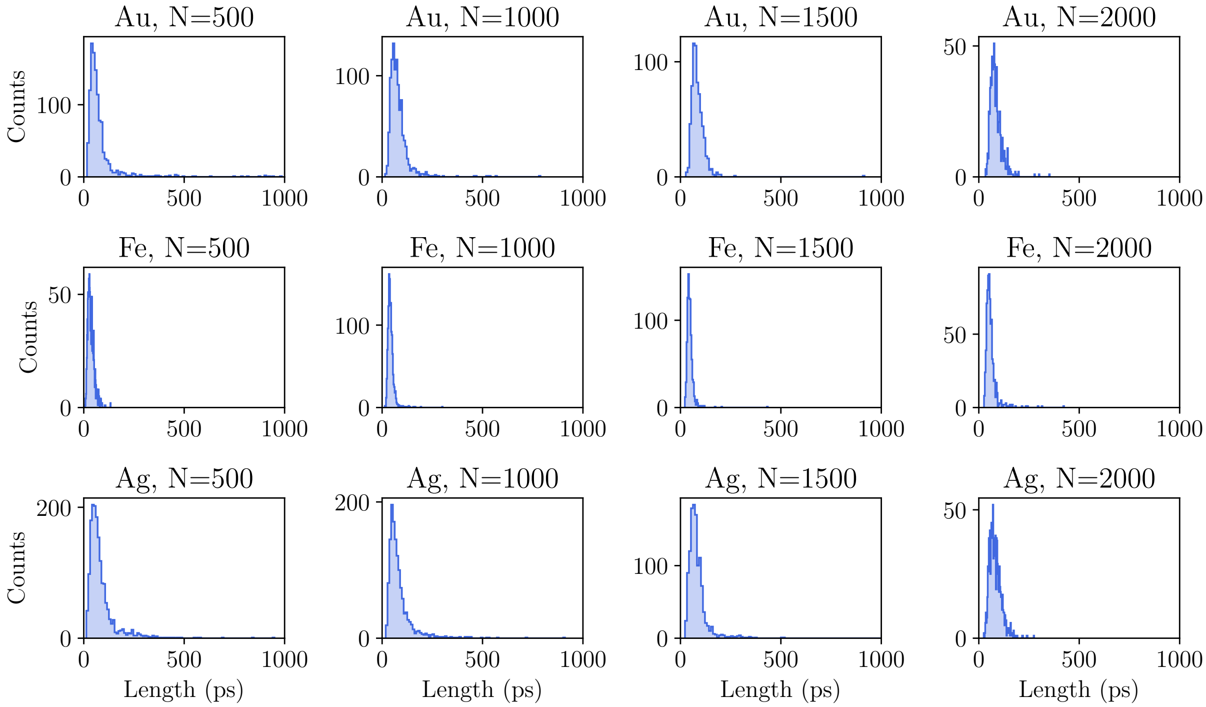


Figure S2: Accepted trajectory length distributions of the aimless shooting simulations.

## 3 Influence of *ad hoc* parameters

In order to assess the influence of *ad hoc* parameters, we tested two additional, different values of the cutoff used when computing the Steinhardt's order parameters. We note that because $\overline{q_6}$ measures the degree of symmetry, by increasing the cutoff one blurs the overall symmetry thus reducing the value of $\overline{q_6}$. Fig. S4 shows that as expected, increasing the cutoff leads to a decrease in $N_{crys}$. Yet, the observed behavior is consistent for all values tested.

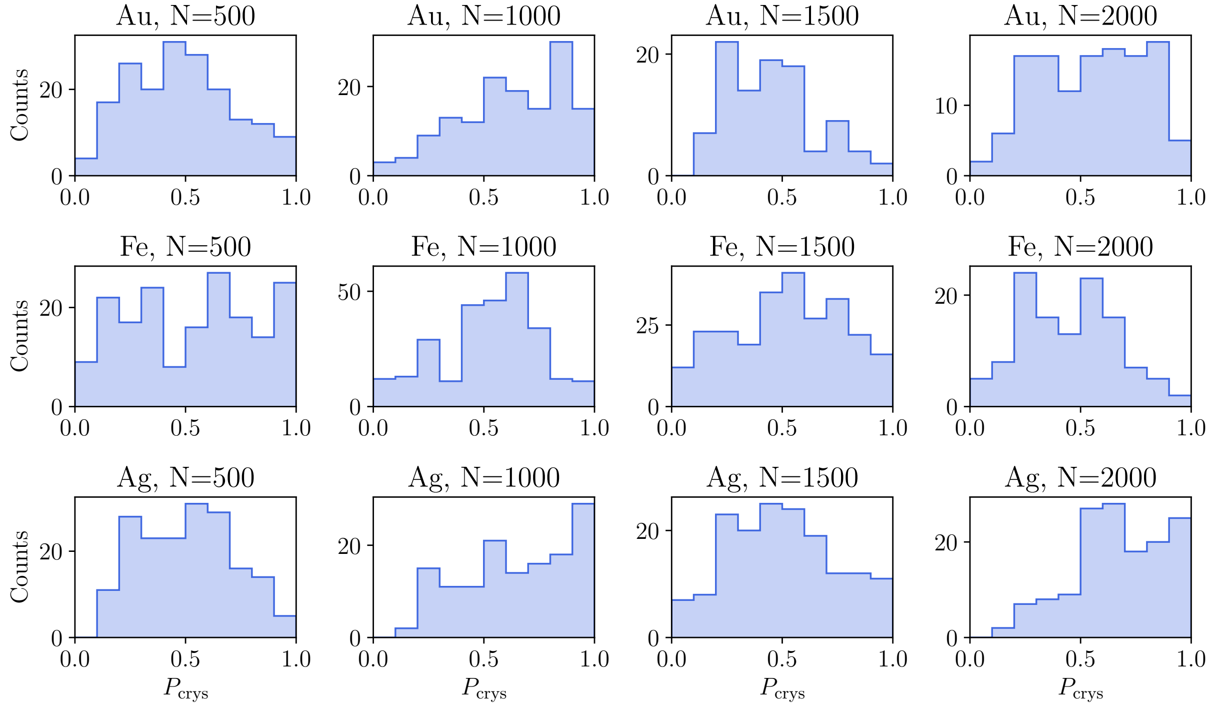


Figure S3: Committor distributions of the structures sampled from aimless shooting simulations.

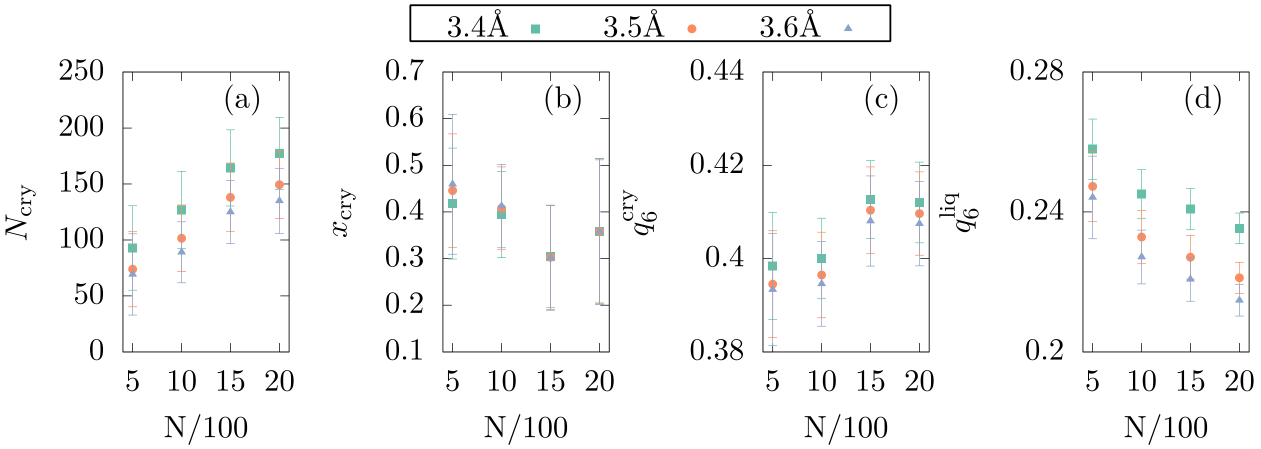


Figure S4: Influence of the droplet size on the structure of the critical structures for gold in terms of the size of the largest crystalline cluster (a), the radial position of the largest crystalline cluster (b), the value of $\overline{q_6}$ averaged over atoms of the largest crystalline cluster (c) and of the remaining atoms (d). Results are obtained with gold using three different values of cut-off for the Steinhardt's order parameters.
